# Supplementary material for: Coherence time of over a second in a telecom-compatible quantum memory storage material
Source: arXiv:1611.04315 ancillary file (2018-04-26)
Supplement: Supplementary file 1 [file Supplementary_materials.pdf]

# Supplementary materials

10 August 2017

## 1 Experimental Diagram

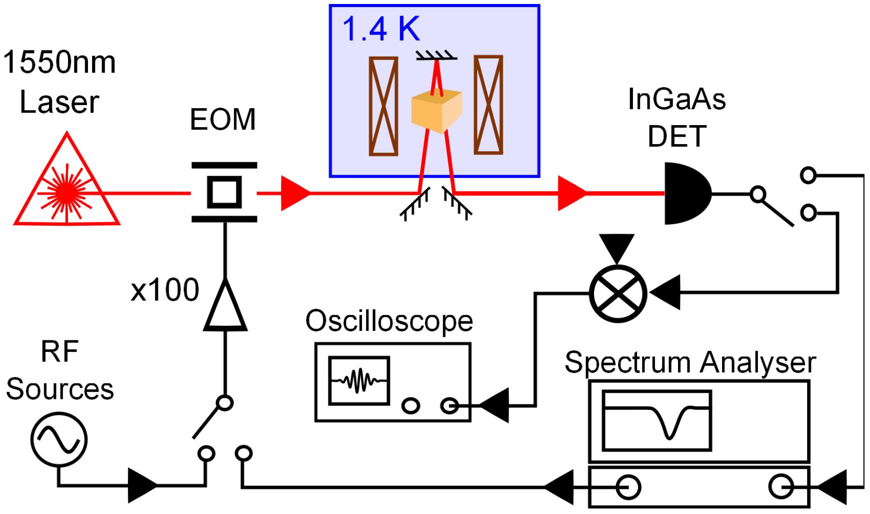


Figure 1: The combined experimental setup for all measurements recorded. In all cases, the light source used was a single frequency stabilized laser and two optical sidebands generated by either an amplitude or phase modulating EOM. A series of TTL RF switches were used to alternate between RF sources (and measurement devices). Three tunable single-frequency RF sources were available to generate short optical pulses as well as a VCO for hyperfine spin-pumping. Most spectra were recorded on the spectrum analyser using AM spectroscopy. Echo measurements were recorded on the oscilloscope by mixing GHz optical modulation and RF to generate a 10 MHz signal.

## 2 The energy level structure of $^{167}Er^{3+} : Y_2SiO_5$

Figure 2 shows the level structure of $^{167}Er^{3+} : Y_2SiO_5$. The crystal field splits the atomic Er states into Kramers doublets. The degeneracy of these 'effective' spin-1/2 pairs can only be lifted by applying a magnetic field. In this work, a magnetic field of 7 T creates a 1.1 THz splitting of the lowest Kramers doublet of the $^4I_{15/2}$ multiplet. We investigated the properties of the ground state hyperfine structure by exciting the optical transition between the 'spin-down' projections of the lowest Kramers doublets in each of the $^4I_{15/2}$ and $^4I_{13/2}$ multiplets. This optical transition occurs at 1538 nm.

## 3 Measurement of the hyperfine structure

With eight hyperfine states in both the ground and excited state, the holeburning structure of this system is very complicated. Additionally, because the different transitions making up each of the $\Delta m_I = 0, \pm 1$ absorption bands are partly resolved, only a subset of the possible holeburning structure is observed when burning in any particular part of an absorption band. Therefore, we burnt many holes across the $\Delta m_I =$

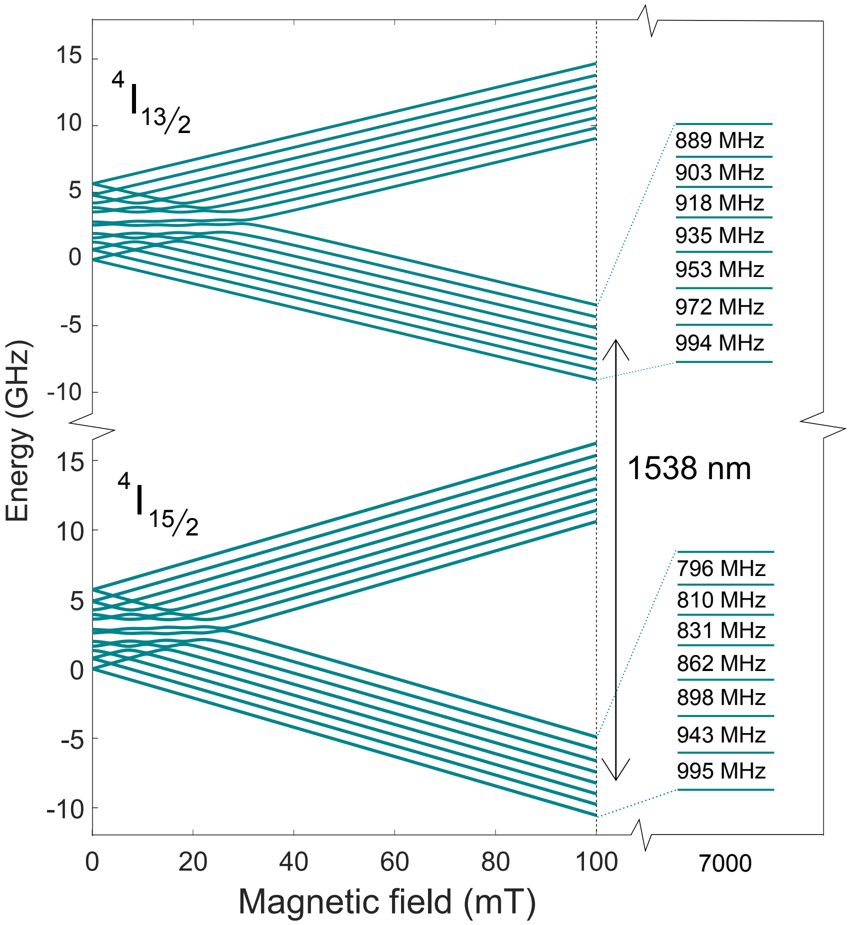


Figure 2: An energy level diagram of $^{167}Er^{3+}$ : $Y_2SiO_5$. **The left side** shows the splitting of the 16 hyperfine states in the lowest Kramers doublets of the ground $^4I_{15/2}$ and excited $^4I_{13/2}$ states. The structure of the $I_{15/2}$ doublet is determined from an effective spin-hamiltonian[1]. The $^4I_{13/2}$ structure has not been experimentally determined, and an indicative approximation is given that makes use of the calculated Zeeman splitting from the crystal field Hamiltonian [2]. **The right side** shows the hyperfine structure of the lower Zeeman arms of the two Kramers doublets at 7T.

$0, +1$ transitions to determine all the hyperfine splittings and correctly assign them to levels. Using this method, it was possible to determine all the hyperfine splittings to within 5 MHz. We also burnt holes in the $\Delta m_I = 0$ band after the ensemble had been spin pumped to check the splitting assignments.

For all holeburning measurements, the laser frequency was approximately 2 GHz blue-detuned from the transition and one sideband of the EOM (see paper) was used to burn holes across the $\Delta m_I = 0$ or $\Delta m_I = +1$ absorption bands in 100 MHz increments. For spin pumping measurements, holes were burnt in the $\Delta m_I = 0$ bands in the same way after the ensemble had been partially spin polarized towards the $m_I = |{+}^7\!/_2\rangle$ hyperfine ground state using the method described in the paper. The hole structure generated was then read out by sweeping the EOM sideband across the line.

An example holeburning spectrum from the spin-pumped dataset is shown in Figure 3. The central hole, labelled **H**, was burnt at approximately 500 MHz into a population mostly consisting of atoms in the $|{+}^7\!/_2\rangle$ hyperfine ground state, with some in the $|{+}^5\!/_2\rangle$. Anti-holes associated with the central hole are visible both in the $\Delta m_I = 0$ and $\Delta m_I = +1$ absorption bands.

## 4 Comparison with the zero field spin-Hamiltonian

A common way of modelling the hyperfine structure of a single electronic state in a rare earth ion is to use a reduced spin Hamiltonian, which assumes a static contribution of the electronic level to the hyperfine structure. This approach has been taken for the $^4I_{15/2}$ ground state of Er at low field [3] and has been used

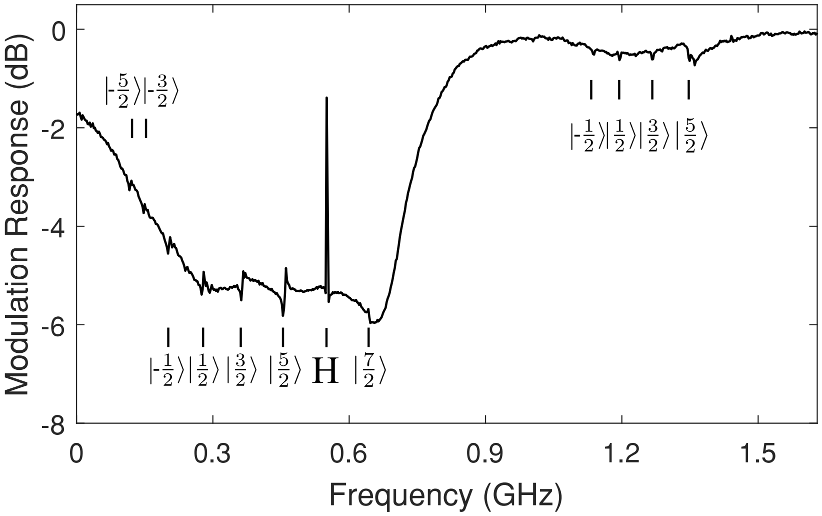


Figure 3: The optical absorption spectrum obtained by AM spectroscopy after a spectral hole **(H)** is burnt at 500 MHz in the figure. After hole-burning, there is a distinct pattern of anti-holes in the $\Delta m_I = 0$ and $+1$ absorption bands. The dispersive lineshape of the anti-holes is a consequence of spectral diffusion. Labeled above and below the anti-holes are the $^4I_{15/2}$ hyperfine ground states of the transitions.

| Hyperfine transition | Measured (MHz) | Calculated (MHz) |
|---|---|---|
| $-\frac{7}{2} \leftrightarrow -\frac{5}{2}$ | 995 | 801 |
| $-\frac{5}{2} \leftrightarrow -\frac{3}{2}$ | 943 | 773 |
| $-\frac{3}{2} \leftrightarrow -\frac{1}{2}$ | 896 | 784 |
| $-\frac{1}{2} \leftrightarrow \frac{1}{2}$ | 862 | 800 |
| $\frac{1}{2} \leftrightarrow \frac{3}{2}$ | 831 | 814 |
| $\frac{3}{2} \leftrightarrow \frac{5}{2}$ | 810 | 836 |
| $\frac{5}{2} \leftrightarrow \frac{7}{2}$ | 796 | 890 |

Table 1: $^4I_{15/2}$ ground state hyperfine splittings measured in this work compared with those calculated from the published reduced spin Hamiltonian of Guillot-Noël et al. [3]

to estimate ZEFOZ point positions [4]. The resulting Hamiltonian can be used to calculate the expected hyperfine splittings at the 7T field we studied. These splittings are shown in comparison to the measured values in Table 1.

These theoretical hyperfine splittings are only correct to within 15%, and have an inverted gradient of energies compared to our measured values. This comes about because the assumption that the electronic contribution to the hyperfine splittings is static only holds in a Kramers system over very small magnetic field ranges. In fact, the mixing of the electronic levels changes substantially over 0–7 T, and an effective spin Hamiltonian is not applicable over such a broad range of fields. A more accurate model of the hyperfine structure requires taking the crystal field mixing into account[2]. Such a model will be required to calculate accurate ZEFOZ points for this crystal.

# 5 Hyperfine population rate equations

Once the hyperfine spin ensemble is polarized into the $m_I = |{+}7/2\rangle$ state, it thermally depolarizes by coupling to the crystal lattice. We used a set of coupled rate equations to model this process. This model had a common coupling factor $\gamma$ between levels with $\Delta m_I = \pm 1$, and no coupling between levels with $\Delta m_I > 1$, since these transitions are sufficiently weak that they will not substantially contribute to the decay dynamics. This means that the outer two levels, $m_I = |\pm 7/2\rangle$, are coupled to only a single state,

and are described by a rate equation:

$$\frac{dN(t)_{\pm 7/2}}{dt} = -\gamma \left(N(t)_{\pm 7/2} - N(t)_{\pm 5/2}\right) \quad (1)$$

All other states are coupled to two other levels, so for $m_I = \{-5/2, \ldots, 5/2\}$, the rate equation is

$$\frac{dN(t)_{m_I}}{dt} = -\gamma \left(2N_{m_I}(t) - N_{m_I-1}(t) - N_{m_I+1}(t)\right) \quad (2)$$

The decay constant $\gamma$ encapsulates all the spin-lattice processes described in the text. Because the relative contribution of each process depends on temperature, $\gamma$ is also temperature dependent. The physical significance of $\gamma$ is that $\frac{1}{\gamma}$ is identical to the population decay rate $T_1$ for the $m_I = |\pm {}^7\!/\!_2\rangle$ states, while $T_1 = \frac{1}{2\gamma}$ for $m_I = \{-5/2, \ldots, 5/2\}$.

To determine $\gamma(T)$ for each temperature, the population was spin pumped towards the $m_I = |{+}{}^7\!/\!_2\rangle$ hyperfine ground state and a time series of spectra was recorded as the population relaxed using AM spectroscopy. An example is shown in Figure 4. The model was fitted to the first spectrum (10 second delay) to determine the distribution of the initial hyperfine population $N_{m_I}(0)$. This was necessary as the efficiency of the spin pumping is also temperature-dependent. The model was then fitted to the remaining spectra to determine $\gamma$. These fits are shown in Figure 4.

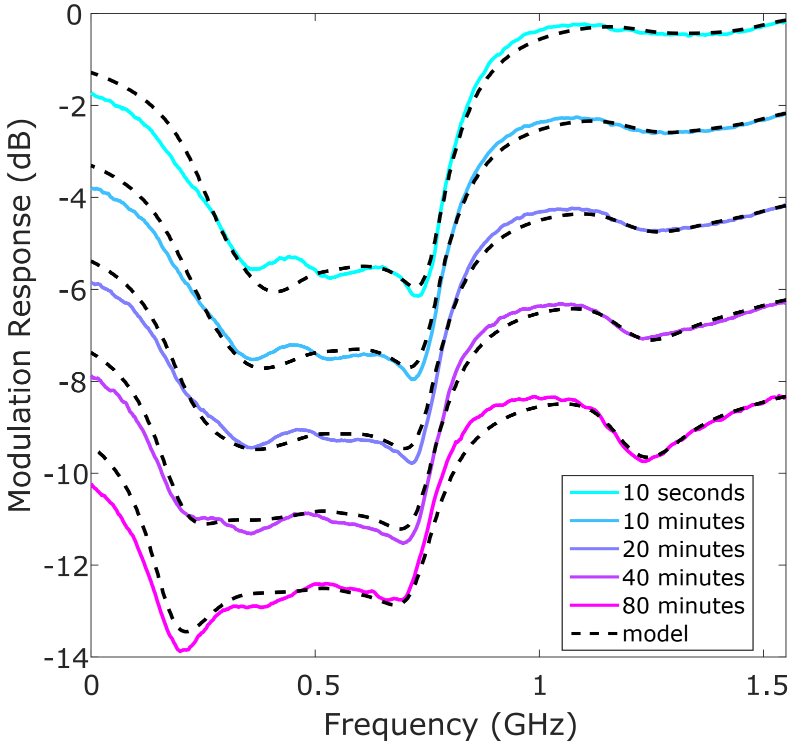


Figure 4: The colored traces are the time series of spectra recorded at 1.6 K following hyperfine spin pumping. The black dashed traces show the fitting of the population model for each delay. Our method focused on accurately fitting the $\Delta m_I = +1$ transitions between 1-1.5 GHz, rather than the $\Delta m_I = 0$ transitions. For this reason the model does not match the data as well for low frequencies.

## 6 Decoherence caused by Yttrium spin-flips

The dominant source of decoherence on the Er transition is spin-flips of the Y spin bath. This can be considered to consist of a frozen core of Y spins around each dopant ion, whose transition frequencies are detuned by the large magnetic field generated by the Er ion and so flip slowly, and the bulk ions outside this core, which are unaffected by the Er ion. Modelling the frozen core dynamics is challenging, but an upper

estimate of the contribution of the Y atoms to the Er decoherence can be obtained by ignoring the frozen core. This treatment relies on the assumption that the Y spin flips are rapid relative to the Er decoherence rate so that the perturbation due to the Y spin bath is maximal. This is reasonable in $Er^{3+} : Y_2SiO_5$. since the bulk spin flip rate is 8 Hz [5]. The decoherence due to the spin flips of the bulk Y ions can then be estimated to first order as [6, 7]:

$$\frac{1}{\pi T_2} = \nabla f \cdot \Delta \mathbf{B} \tag{3}$$

where$\nabla f$ is the gradient of the hyperfine transition frequency and $\Delta \mathbf{B}$ is the FWHM of the magnetic field fluctuations caused by the bulk Y ions, which is $8\mu$T in $Y_2SiO_5$ [7]. We measure the transition gradient along the $D_1$ axis, $\frac{\partial f}{\partial B} = 11$ MHz/T, and from equation (3) we obtain an upper bound for the coherence time of 3.6 ms.

# References


[1] E. Baldit, *et al.* Identification of $\Lambda$ -like systems in $Er^{3+}$:$Y_2SiO_5$ and observation of electromagnetically induced transparency. *Physical Review B*, 81(14):144303 (2010).

[2] Sebastian Horvath. High-resolution spectroscopy and novel crystal-field methods for rare-earth based quantum information processing. *PhD thesis, University of Canterbury* (2016).

[3] Guillot-Noël, O., Goldner, P., Du, Y. L., Baldit, E., Monnier, P., & Bencheikh, K. Hyperfine interaction of $Er^{3+}$ ions in $Y_2SiO_5$: An electron paramagnetic resonance spectroscopy study. *Physical Review B*, 74(21):214409 (2006).

[4] D. L. McAuslan,, Bartholomew, J. G., Sellars, M. J., & Longdell, J. J. Reducing decoherence in optical and spin transitions in rare-earth-metal-ion-doped materials. *Physical Review A*, 85(3):032339 (2012).

[5] Böttger, T., Thiel, C. W., Sun, Y. & Cone, R. L. Optical decoherence and spectral diffusion at 1.5 $\mu$m in $Er^{3+}$:$Y_2SiO_5$ versus magnetic field, temperature, and $Er^{3+}$ concentration. *Physical Review B*, 73(7):075101 (2006).

[6] E. Fraval, M. J. Sellars, and J. J. Longdell. Method of Extending Hyperfine Coherence Times in Pr:Y2SiO5. *Physical Review Letters*, 92(7):077601 (2004).

[7] Manjin Zhong *et al.* Optically addressable nuclear spins in a solid with a six-hour coherence time. *Nature*, 517(7533):177–80 (2015).
